# Supplementary material for: EcoMem: An R package for quantifying ecological memory
Source: arXiv:1902.07706 ancillary file (2019-02-20)
Supplement: Supplementary file 1 [file AppendixA.pdf]

**Article title**: `EcoMem`: An R package for quantifying ecological memory

**Appendix A**: Ecological memory model inference

**Authors**: Malcolm Itter, Jarno Vanhatalo, and Andrew Finley

## Model inference

The ecological memory model is completed by assigning priors for model parameters including regression coefficients $\mu$ and $\boldsymbol{\beta}$, basis function coefficients $\boldsymbol{\eta}_j$'s, regulator parameters $\tau_j^2$'s, and the residual variance ($\sigma_y^2$). As noted in the main text, basis function coefficients are assigned a weakly informative normal prior dependent on a regulator parameter and penalty matrix: $\boldsymbol{\eta}_j \sim \text{N}(\mathbf{0}, \tau_j^2 \mathbf{S}_j^-)$. The square root of regulator parameters are assigned independent, folded $t$ distributions: $\tau_j \sim \text{Folded-}t(A, \nu)$. Using the parameterization for the folded $t$ distribution presented in Gelman et al. (2006), we set the scale parameter ($A$) and the degrees of freedom ($\nu$) equal to 0.1 and 4, respectively, placing high prior density on small $\tau_j$ values. For notational and sampling convenience, we include $\mu$ within the regression coefficients $\boldsymbol{\beta}$, which are assigned a normal prior distribution: $\boldsymbol{\beta} \sim \text{N}(\mathbf{0}, \sigma_\beta^2 \mathbf{I})$ with $\sigma_\beta^2 =$ 1E07. Finally, the residual standard deviation is assigned a uniform prior: $\sigma_y \sim \text{Unif}(a_y, b_y)$ with $a_y =$ 1E-07 and $b_y =$ 1E07.

Combining the likelihood, estimation of latent weights (i.e., ecological memory functions), and prior distributions, the joint posterior distribution is given by,

$$\begin{aligned}\boldsymbol{\beta}, \boldsymbol{\eta}, \boldsymbol{\tau}^2, \sigma_y^2 | \mathbf{y} \propto p(\mathbf{y} | g^{-1}(\tilde{\mathbf{X}}\boldsymbol{\beta}), \sigma_y^2) \times \text{N}(\boldsymbol{\beta}|\mathbf{0}, \sigma_\beta^2 \mathbf{I}) \times \prod_{j=1}^{p_\text{m}} \text{N}(\boldsymbol{\eta}_j | \mathbf{0}, \tau_j^2 \mathbf{S}_j^-) \times \\ \prod_{j=1}^{p_\text{m}} \text{Folded-}t(\tau_j | A, \nu) \times \text{Unif}(\sigma_y | a_y, b_y)\end{aligned} \quad \text{(A.1)}$$

using notation similar to Hobbs and Hooten (2015). In Eq. (A.1), $\mathbf{y}$ is an $n$-dimesional vector of observed response values, $\boldsymbol{\beta}$ is a $(p+1)$-dimensional vector of regression coefficients (includes $\mu$), $\tilde{\mathbf{X}}$ is an $n \times (p+1)$ design matrix including an intercept term and weighted covariates values for each memory function variable, $\boldsymbol{\eta}_j$ is a $k_j$-dimensional vector of basis function coefficients for $j = 1, 2, \ldots, p_\text{m}$, with $p_\text{m}$ equal to the total number of memory function variables in the model ($p_\text{m} \leq p$), $k_j$ is the number of knots used to estimate the $j$th memory function, and $\mathbf{S}_j$ is a $k_j \times k_j$ matrix of known coefficients based on knot placement. Likelihood functions are denoted by $p(\cdot)$ and $g^{-1}(\cdot)$ indicates the inverse of the applied link function (Table A.1). The $\sigma_y^2$ term is only included if the likelihood is Gaussian.

Table A.1: List of likelihood and link functions used to estimate ecological memory.

| Likelihood function | Link function | $g(x)$ |
|---|---|---|
| Gaussian | Identity | $x$ |
| Poisson | Log | $\log x$ |
| Binomial | Logit | $\log \frac{x}{1-x}$ |

## Gibbs sampler

We use a Metropolis-within-Gibbs Markov chain Monte Carlo (MCMC) algorithm (Robert and Casella, 2004) to sample from the posterior distribution in Eq. (A.1). An elliptical slice sampler is used to update basis function coefficient values. All other model parameters are updated directly when possible, otherwise an adaptive Metropolis update is applied (Roberts and Rosenthal, 2009). We provide full conditional distributions for each Gibbs step and details on elliptical slice and Metropolis updates (including log-target densities) below.

### Update $\boldsymbol{\beta}$

Gaussian likelihood:

$\boldsymbol{\beta}|\cdot \sim \mathrm{N}(\mathbf{V}\mathbf{v}, \mathbf{V})$ where

$$\mathbf{V} = \left(\frac{\tilde{\mathbf{X}}'\tilde{\mathbf{X}}}{\sigma_y^2} + \frac{\mathbf{I}_p}{\sigma_\beta^2}\right)^{-1}$$
$$\mathbf{v} = \frac{\tilde{\mathbf{X}}'\mathbf{y}}{\sigma_y^2}$$

Non-Gaussian likelihood:

Regression coefficients $\boldsymbol{\beta}$ are updated individually by proposing a new value from a normal distribution centered on the current value. The new value for $\beta_j$ is used to update the mean response, $g^{-1}(\tilde{\mathbf{X}}\boldsymbol{\beta})$, and accepted or rejected based on the following log-target densities,

*Poisson*:

$$l(\beta_j|\cdot) \propto \mathbf{y}'(\tilde{\mathbf{X}}\boldsymbol{\beta} + \log \mathbf{o}) - (\exp(\tilde{\mathbf{X}}\boldsymbol{\beta}))'\mathbf{o} - \frac{1}{2\sigma_\beta^2}\boldsymbol{\beta}'\boldsymbol{\beta}$$

*Binomial*:

$$l(\beta_j|\cdot) \propto \mathbf{y}' \log\left(\frac{1}{1+\exp(-\tilde{\mathbf{X}}\boldsymbol{\beta})}\right) + (\mathbf{o}-\mathbf{y})' \log\left(\frac{\exp(-\tilde{\mathbf{X}}\boldsymbol{\beta})}{1+\exp(-\tilde{\mathbf{X}}\boldsymbol{\beta})}\right) - \frac{1}{2\sigma_\beta^2}\boldsymbol{\beta}'\boldsymbol{\beta}$$

where $\mathbf{o}$ is an $n$-dimensional vector of offset or number of trial values for Poisson and binomial data, respectively.

### Update $\boldsymbol{\eta}_j$ $(j = 1, \ldots, p_m)$

An elliptical slice sampler is used to update the basis function coefficients used to estimate ecological memory weights per Eq. (4) in the main article (Murray et al., 2010). Use of an elliptical slice sampler allows for joint updates of $\boldsymbol{\eta}_j$ despite the high correlation among individual basis function coefficients, which can lead to poor mixing of chains and slow convergence. Steps to update $\boldsymbol{\eta}_j$ using an elliptical slice sampler are as follows (adapted from Murray et al., 2010).

1. Set a log-likelihood threshold ($\alpha$) equal to $l(\mathbf{y}) + \log u$ where $u \sim \text{Unif}[0,1]$ and $l(\mathbf{y})$ depends on the type of response,

   *Gaussian*: $l(\mathbf{y}) \propto -\frac{1}{\sigma_y^2}(\mathbf{y} - \tilde{\mathbf{X}}\boldsymbol{\beta})'(\mathbf{y} - \tilde{\mathbf{X}}\boldsymbol{\beta})$

   *Poisson*: $l(\mathbf{y}) \propto \mathbf{y}'(\tilde{\mathbf{X}}\boldsymbol{\beta} + \log \mathbf{o}) - (\exp(\tilde{\mathbf{X}}\boldsymbol{\beta}))'\mathbf{o}$

   *Binomial*: $l(\mathbf{y}) \propto \mathbf{y}' \log\left(\frac{1}{1+\exp(-\tilde{\mathbf{X}}\boldsymbol{\beta})}\right) + (\mathbf{o} - \mathbf{y})' \log\left(\frac{\exp(-\tilde{\mathbf{X}}\boldsymbol{\beta})}{1+\exp(-\tilde{\mathbf{X}}\boldsymbol{\beta})}\right)$

2. Propose an ellipse ($\boldsymbol{\xi}$) by sampling from the prior distribution for $\boldsymbol{\eta}_j$: $\boldsymbol{\xi} \sim \text{N}(\mathbf{0}, \tau_j^2 \mathbf{S}_j^-)$

3. Draw a proposal angle: $\theta \sim \text{Unif}[0, 2\pi]$, defining an initial search bracket: $\theta_{\text{min}} = \theta - 2\pi$; $\theta_{\text{max}} = \theta$

4. Generate a proposal value for $\boldsymbol{\eta}_j$: $\boldsymbol{\eta}_j^* = \boldsymbol{\eta}_j \cos\theta + \boldsymbol{\xi} \sin\theta$

5. Update values for $\mathbf{w}_j$ and $\tilde{\mathbf{X}}$ based on $\boldsymbol{\eta}_j^*$ and calculate $l(\mathbf{y})^*$ using new $\tilde{\mathbf{X}}$ matrix

6. If $l(\mathbf{y})^* > \alpha$, accept $\boldsymbol{\eta}_j^*$ (STOP), else shrink the search bracket: if $\theta < 0$, $\theta_{\text{min}} = \theta$, else $\theta_{\text{max}} = \theta$

7. Draw a new angle: $\theta \sim \text{Unif}[\theta_{\text{min}}, \theta_{\text{max}}]$

8. Return to step (4)

In the current MCMC implementation, the elliptical slice sampler is run multiple times (defined by the `n.step` argument to the `ecomem()` and `ecomemGLM()` functions) per MCMC iteration to speed convergence.

**Update** $\tau_j$ $(j = 1, \ldots, p_m)$

The scalar penalty on the basis function coefficients ($\tau_j^2$) controls the smoothness of ecological memory functions. We choose to assign a prior to the square root of the penalty parameter ($\tau_j$) similar to estimating variance parameters in hierarchical models (Gelman et al., 2006). The square root of the penalty parameter is updated by proposing a new value from a normal distribution centered on the log-transformed current value of $\tau_j$. The new value for $\tau_j$ is accepted or rejected using the following log-target density (the parameterization of the folded-$t$ distribution appearing in the log-target density comes from Gelman et al., 2006),

$$l(\tau_j|\cdot) \propto -(k_j - 1)\log\tau_j - \frac{1}{2\tau_j^2}\boldsymbol{\eta}_j'\mathbf{S}_j\boldsymbol{\eta}_j - \frac{\nu+1}{2}\log\left(1 + \frac{1}{\nu}\left(\frac{\tau_j}{A}\right)^2\right).$$

**Update** $\sigma_y$

The residual standard deviation $\sigma_y$, estimated only for Gaussian response data, is updated by proposing a new value from a normal distribution centered on the logit-transformed current value of $\sigma_y$. Note, the logit transformation defined for the standard deviation, $f(\sigma_y) =$

$\log\left(\frac{\sigma_y - a_\sigma}{b_\sigma - \sigma_y}\right)$, is not the same as the logit link function. The new value for $\sigma_y$ is accepted or rejected based on the following log-target density,

$$l(\sigma_y|\cdot) \propto -n \cdot \log(\sigma_y) - \frac{1}{2\sigma_y^2}(\mathbf{y} - \tilde{\mathbf{X}}\boldsymbol{\beta})'(\mathbf{y} - \tilde{\mathbf{X}}\boldsymbol{\beta}) + \log(\sigma_y - a_y) + \log(b_y - \sigma_y).$$

# References


Gelman, A. et al. (2006). Prior distributions for variance parameters in hierarchical models (comment on article by Browne and Draper). *Bayesian Analysis*, 1(3):515–534.

Hobbs, N. T. and Hooten, M. B. (2015). *Bayesian Models: A Statistical Primer for Ecologists*. Princeton University Press.

Murray, I., Prescott Adams, R., and MacKay, D. J. (2010). Elliptical slice sampling. *Journal of Machine Learning Research*, 9:541–548.

Robert, C. and Casella, G. (2004). *Monte Carlo Statistical Methods*. Springer Texts in Statistics. Springer-Verlag, New York.

Roberts, G. O. and Rosenthal, J. S. (2009). Examples of adaptive MCMC. *Journal of Computational and Graphical Statistics*, 18(2):349–367.
