# Supplementary material for: EcoMem: An R package for quantifying ecological memory
Source: arXiv:1902.07706 ancillary file (2019-02-20)
Supplement: Supplementary file 2 [file AppendixB.pdf]

**Article title**: `EcoMem`: An R package for quantifying ecological memory

**Appendix B**: Annotated code for simulated and applied case study examples

**Authors**: Malcolm Itter, Jarno Vanhatalo, and Andrew Finley

## Overview

The `EcoMem` package estimates ecological memory functions for a specified subset of covariates implementing the Bayesian hierarchical framework defined in Section 2 of the main article. The package currently accommodates continuous, count, and proportional response observations and continuous and binary covariate observations. We demonstrate the functionality of the `EcoMem` package to make advanced ecological inference through its application to a simulated Poisson data set and a case study assessing the ecological memory of boreal tree growth to insect defoliation events.

## Installation

The development version of `EcoMem` is available on GitHub and can be installed using `devtools` (Wickham et al., 2018). A list of the core functions available within `EcoMem` is provided in Table 1 of the main article.

```
# Install EcoMem package
devtools::install_github("msitter/EcoMem")
library(EcoMem)
```

Additional packages needed for the applied examples are loaded below.

```
library(plyr)
library(kableExtra)
library(ggplot2)
```

## Simulated example

### Simulate from ecological memory model

As an introduction to `EcoMem`, we simulate Poisson count data for $n$ time points, $\mathbf{y} \sim \text{Poisson}(\boldsymbol{\lambda})$, where $\boldsymbol{\lambda}$ is the intensity, from the ecological memory model defined in the main article, then recapture model parameters applying the `ecomemGLM()` function. The intensity is generated applying a log link function of three covariates, $\mathbf{v}_1, \mathbf{v}_2, \mathbf{v}_3$ as,

$$\log \boldsymbol{\lambda} = \beta_0 \mathbf{1} + \beta_1 \mathbf{v}_1 + \beta_2 \mathbf{v}_2 + \beta_3 \mathbf{v}_3 + \beta_4 \mathbf{v}_1 \backslash * \mathbf{v}_2 + \beta_5 \mathbf{v}_2 \backslash * \mathbf{v}_3,$$

where $\boldsymbol{\beta} \equiv (\beta_0, \beta_1, \ldots, \beta_5)'$ comprises the regression coefficients, $\mathbf{1}$ is an $n$-dimensional vector of ones, and "$\backslash *$" indicates element-wise multiplication. The $\mathbf{v}_1$ and $\mathbf{v}_2$ variables represent

memory covariates to which the simulated response exhibits memory for up to 10 and 6 time points, respectively ($L_1 = 10, L_2 = 6$). The $\mathbf{v}_3$ variable is an auxiliary covariate. We simulate covariate values for $n = 500$ time points for five independent groups. Let us first define a data frame (`mem.dat`) to house the model variables.

```
# Set data parameters
n = 500
L = c(10,6)
TT = n + max(L)
n.grp = 5
groups = 1:n.grp

# Define model data frame
mem.dat = data.frame(time = rep(1:TT, n.grp),
                     group = rep(groups, each = TT))
```

Next, we simulate values for the three covariates ($\mathbf{v}_1, \mathbf{v}_2, \mathbf{v}_3$). The $\mathbf{v}_1$ covariate is binary representing discrete events over time (e.g., a disturbance chronology). All other covariates are continuous. Covariate values are simulated using a temporally-varying mean with low temporal autocorrelation and minimal correlation among covariates.

```
# Set random seed
set.seed(1)

# Simulate covariate v1
mem.dat$v1 = rbinom(n.grp*TT, 1, rep(0.01+(1:TT)/(8*TT), n.grp))

# Similate covariate v2
mem.dat$v2 = scale(0.4*rgamma(n.grp*TT, shape = 10, scale = 2) +
                     0.6*rnorm(n.grp*TT, sin(8*pi*(1:TT)/TT), 4))

# Simulate covariate v3
int3 = runif(n.grp, -0.5, -0.1)
sd3 = runif(n.grp, 0.6, 1.2)
mem.dat$v3 = scale(as.vector(sapply(1:n.grp, function(i){
  rnorm(TT, int3[i]+0.1*cos(4*pi*(1:TT)/TT), sd3[i])
})))

# Define interaction terms
mem.dat$v1.v2 = with(mem.dat, v1*v2)
mem.dat$v2.v3 = with(mem.dat, v2*v3)

# Check correlation among covariates
cor(mem.dat[,c("v1","v2","v3","v1.v2","v2.v3")])

##                   v1            v2            v3         v1.v2         v2.v3
```

```
## v1      1.000000000 -0.001716984  0.061410925 -0.005559191  0.01552493
## v2     -0.001716984  1.000000000 -0.017227837  0.284631840 -0.02224091
## v3      0.061410925 -0.017227837  1.000000000  0.009939873  0.01212473
## v1.v2 -0.005559191  0.284631840  0.009939873  1.000000000  0.05295884
## v2.v3  0.015524926 -0.022240910  0.012124732  0.052958837  1.00000000
```

Ecological memory weights for variables $\mathbf{v}_1$ and $\mathbf{v}_2$ are generated using modified Gompertz and exponential decay functions, respectively.

```
# Define modified Gompertz decay function
gf = function(a,b,c,x){
  a*exp(-b*exp(c*x))
}

# Define exponential decay function
ed = function(phi,x){
  exp(-phi*x)
}

# Define weights

# v1
a = 1; b = 1e-02; c = 0.8
w1 = gf(a,b,c,0:L[1])/sum(gf(a,b,c,0:L[1]))

# v2
phi = 1
w2 = ed(phi,0:L[2])/sum(ed(phi,0:L[2]))
```

Ecological memory weights are used to construct weighted versions of variables $\mathbf{v}_1$ and $\mathbf{v}_2$.

```
# Form matrix of lagged v1 values for each time point
v1.lag = do.call("rbind", lapply(1:n.grp, function(i){
  x = mem.dat[mem.dat$group==i,"v1"]
  vals = t(sapply(1:n, function(j){
    x[(L[1]+1):1 + j - 1]
  }))
  vals = rbind(array(NA, dim=c(max(L),L[1]+1)), vals)
  return(vals)
}))

# Calculate weighted version of v1
v1.tilde = v1.lag%*%w1

# Form matrix of lagged v2 values for each time point
v2.lag = do.call("rbind", lapply(1:n.grp, function(i){
```

```
  x = mem.dat[mem.dat$group==i,"v2"]
  vals = t(sapply(1:n, function(j){
    x[(L[2]+1):1 + j - 1 + max(0,L[1] - L[2])]
  }))
  vals = rbind(array(NA, dim=c(max(L), L[2]+1)), vals)
  return(vals)
}))

# Calculate weighted version of v2
v2.tilde = v2.lag%*%w2
```

Finally, we define the design matrix containing weighted covariates ($\tilde{\mathbf{X}}$), set parameter values for $\boldsymbol{\beta}$, calculate the intensity ($\boldsymbol{\lambda}$), simulate the Poisson response ($\mathbf{y}$), and plot the simulated responses by group for reference (Fig. B.1).

```
# Form X.tilde
X.tilde = cbind(rep(c(rep(NA, max(L)), rep(1, n)), n.grp),
                v1.tilde, v2.tilde, mem.dat$v3,
                v1.tilde*v2.tilde, v2.tilde*mem.dat$v3)
colnames(X.tilde) = c("(Intercept)","v1","v2","v3","v1:v2","v2:v3")

# Set regression coefficient values
beta = c(-0.5,2.3,-1.5,-1,2.7,-0.3)

# Calculate the intensity
lambda = exp(X.tilde%*%beta)

# Simulate Poisson response variable
mem.dat$y = rpois(TT*n.grp, lambda)

# Plot simulated response by group
ggplot(aes(x = time,y = y), data = mem.dat) +
  geom_point(alpha = 0.25, size = 1.2) +
  facet_wrap(~group, ncol = 2, scale = "free") +
  theme_bw()
```

### Fit ecological memory model

The ecological memory model is designed to be run after conducting variable selection. Note, the model framework is particularly sensitive to collinearity among memory covariates (i.e., correlation among memory covariates greater than $\approx 0.65$). The user should have a reason to expect the response of interest to exhibit memory to one or more covariates. In particular, the need to specify a maximum lag value $L$ for each memory covariate requires users to have some *a priori* intuition about the nature of persistent responses to ecological drivers. The model is fit using the `ecomem()` or `ecomemGLM()` functions. Here, we use `ecomemGLM()`

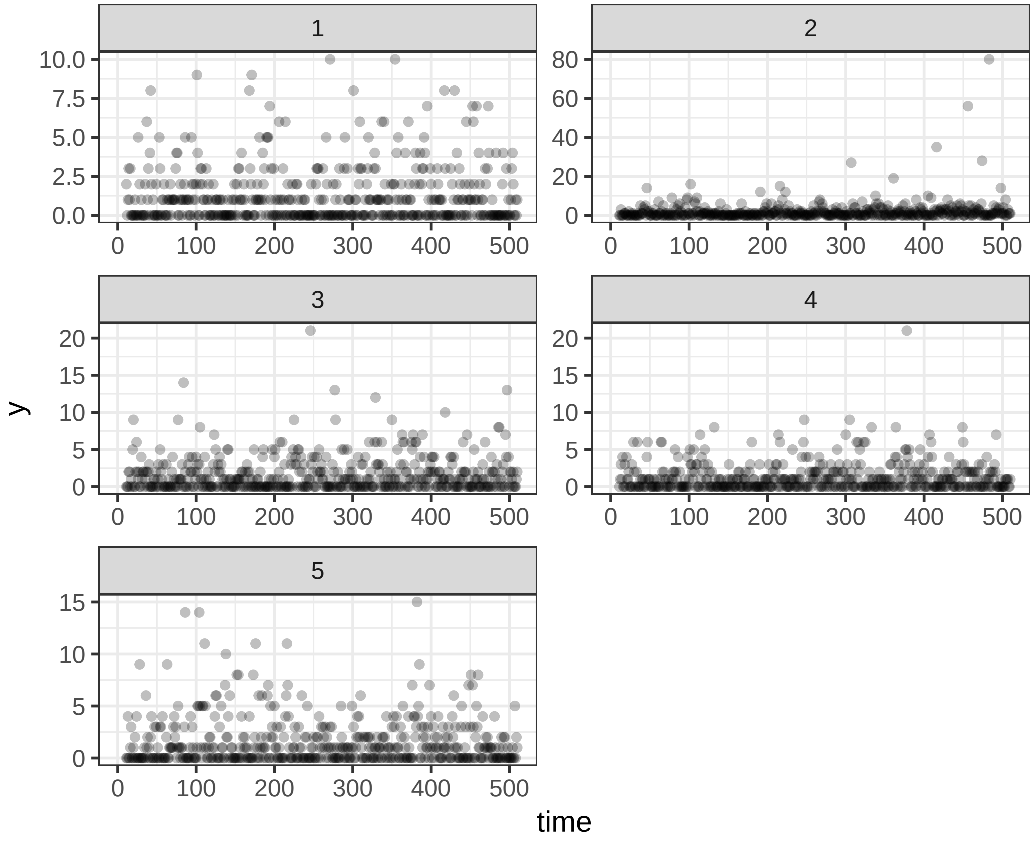


Figure B.1: Simulated Poisson response data by group (note, the y scales are different for each group)

to accommodate the Poisson count data. The `ecomemGLM()` call requires users to specify a linear model `formula`, the likelihood function for the data (`"poisson"` or `"binomial"`), a model data frame including the response, covariates, and all auxiliary variables, a subset of covariates for which memory functions should be estimated, the maximum lag for each memory covariate, as well as time and, if applicable, group identifiers.

```
# Fit ecological memory model
mod = ecomemGLM(y ~ v1*v2 + v2*v3, family = "poisson",
                data = mem.dat, mem.vars = c("v1","v2"),
                L = c(10,6), timeID = "time", groupID = "group")
```

The model is fit using response data for which explanatory variable observations exist for at least `max(L)` previous time points. The default call to `ecomemGLM()` or `ecomem()` fits the ecological memory model applying the Gibbs sampler described in S1 for three MCMC chains run in parallel. Parallelization is implemented using the `snow` and `snowfall` packages (Tierney et al., 2009; Knaus et al., 2009). Alternatively, users can adjust the number of chains (`n.chains = 3`) and/or run the chains in sequence (`parallel = FALSE`). It is also possible to use the `ecomemGLM()` and `ecomem()` functions to generate a list of MCMC inputs (one for each MCMC chain), which can be passed directly into the `ecomemGLMMCMC()` and

`ecomemMCMC()` functions, respectively, for additional user control (`inputs.only = TRUE`). The sampler can be tuned by adjusting the number of posterior samples (`n.post`), thinning interval (`thin`), burn-in period (`burn.in`), and the number of steps taken per iteration by the elliptical slice sampler (`n.step`) used to update ecological memory weights.

### Processing model results

The `ecomemGLM()` and `ecomem()` functions both return a list of class `ecomem` including posterior samples for each MCMC chain (returned only if `inputs.only = FALSE`), the data frame used to fit the model including standardized continuous covariates and responses with `NA` values if covariates are not observed for at least `max(L)` previous time points, and a sample size value indicating the number of response observations used to fit the model. The posterior samples can be converted into an `mcmc` object using the `mem2mcmc()` function allowing users to apply the `coda` package to assess model convergence and summarize results (Fig. B.2; Plummer et al., 2006).

```
# Convert ecomem output to mcmc object
post.samps = mem2mcmc(mod)

# Generate posterior sample traceplots
plot(post.samps[,1:3])
```

The marginal posterior distribution for each ecological memory model parameter can be summarized using the `memsum()` function. The lower and upper quantiles returned as part of the summary can be adjusted using the `cred.int` argument.

```
# Summarize marginal posterior distributions
coef.summ = memsum(mod, cred.int = 0.99, verbose = FALSE)
```

We can compare the marginal posterior distribution of ecological memory parameters to the values used to simulate the data (Fig. B.3).

```
# Add simulation parameter values to coef.summ
coef.summ$sim.val = c(beta,w1,w2)

# Define parameter types (Beta, w1, w2)
coef.summ$var.type = c(rep("Beta", length(beta)),
                       rep("Wts. v1", length(w1)),
                       rep("Wts. v2", length(w2)))

# Determine if simulated parameter value is within credible interval
coef.summ$In = with(coef.summ, ifelse(
  q0.005 < sim.val & q0.995 > sim.val, TRUE, FALSE))

# Convert var to factor
coef.summ$var = factor(coef.summ$var, rev(coef.summ$var))
```

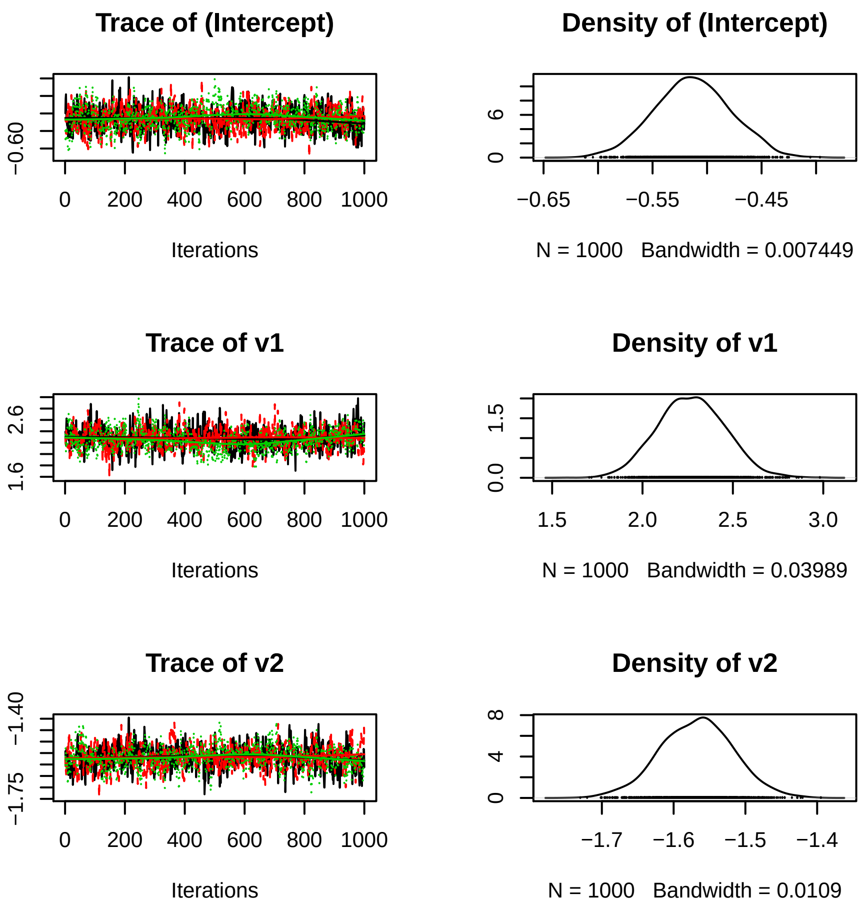


Figure B.2: Traceplots for the `(Intercept)`, `v1`, and `v2` regression coefficients generated using the `plot()` function after converting the `ecomem` model object to a `coda::mcmc` object.

```
# Plot posterior summary of model parameters relative to simulated values
ggplot(aes(x = var, y = mean, ymin = q0.005, ymax = q0.995),
       data = coef.summ) +
  geom_linerange() +
  geom_point(shape = 4, size = 2) +
  geom_point(aes(y = sim.val, color = In),
             size = 2, alpha = 0.6) +
  scale_color_manual(values = c("red","green")) +
  xlab("Parameter") + ylab("Posterior Summary") +
  facet_wrap(~ var.type, ncol = 1, scale = "free") +
  coord_flip() +
  theme_bw() +
  labs(color = "Simulated value in\ncredible interval")
```

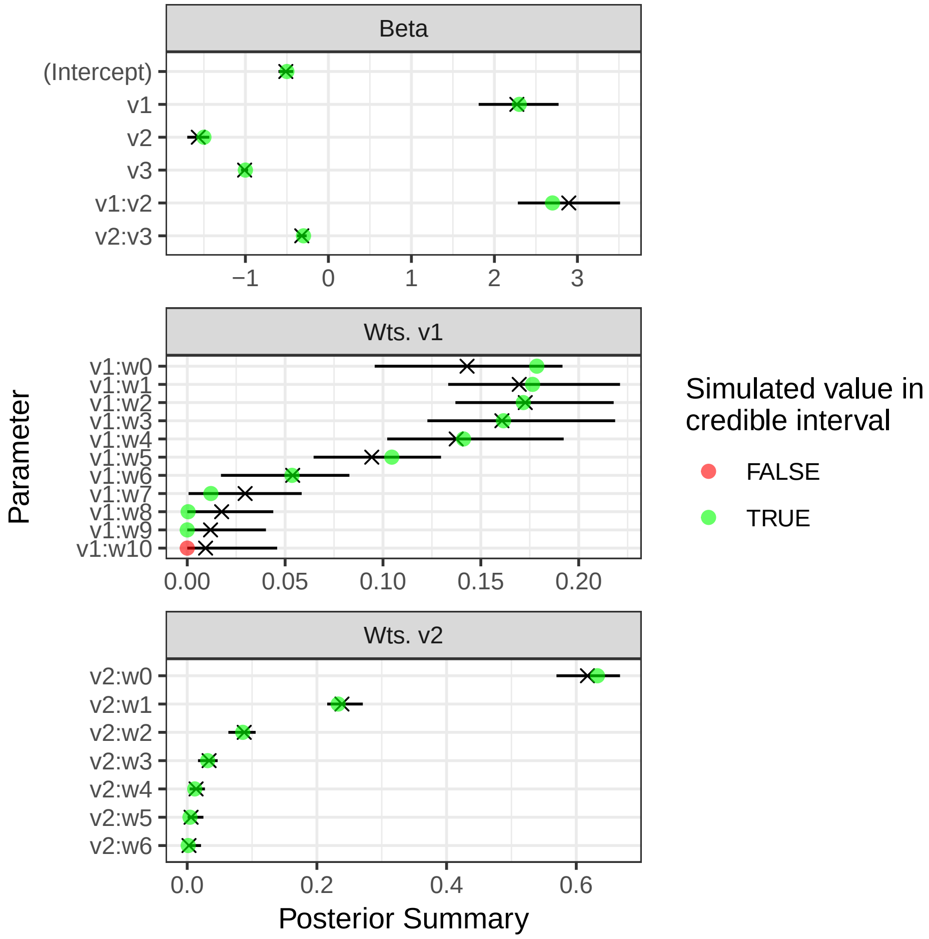


Figure B.3: Posterior mean and credible intervals for ecological memory model parameters (black lines and x symbols) relative to parameter values used to simulate data (colored points).

Finally, ecological memory functions can be plotted for each memory covariate using the `plotmem()` function. We add the weights used to generate the simulated data to the memory function plot for reference (Fig. B.4).

```
# Plot memory functions
p = plotmem(mod, cred.int = 0.99)

# Define data frame with data generating weights
simWts = data.frame(var=rep(paste("v", 1:2, sep = ""), L + 1),
                    lag = unlist(lapply(L, function(x) 0:x)),
                    wt = c(w1,w2))

p + geom_line(inherit.aes = FALSE, data = simWts,
              aes(x = lag, y = wt, color = "Sim. Wts."), size = 0.8) +
  scale_color_manual(values = c("black","darkred"))
```

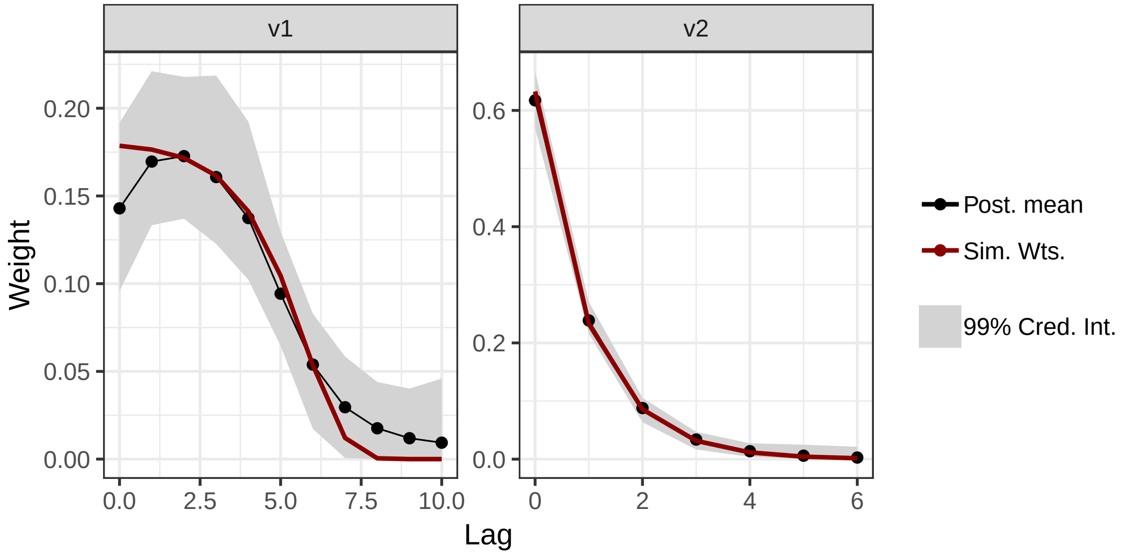


Figure B.4: Ecological memory functions for `v1` and `v2` covariates generated using the `plotmem()` function modified to display the data-generating weight functions for reference.

## Case study - boreal tree growth

As further demonstration of `EcoMem`'s functionality and its utility for ecological inference, we apply the package to forest data from western Canada to assess the memory of boreal tree growth to insect defoliation events. The boreal forest in western Canada is characterized by the interplay of droughts, insect attack, and fire (Brandt et al., 2013). Recent work has shown that boreal tree growth exhibits negative responses to insect defoliation for several years following a moderate-to-severe defoliation event (Itter et al., 2018a). We apply the `EcoMem` functions to annual tree growth and insect defoliation survey data for 34 sites across Alberta, Canada to assess the ecological memory of tree growth to defoliation (see Itter et al. (2018a) for detailed description of dataset). The forest tent catepillar (*Malascosoma disstria* Hub.) is the primary insect defoliator in Alberta feeding on newly-flushed trembling aspen (*Populus tremuloides* Michx.) leaves (Brandt et al., 2013).

The boreal tree growth and defoliation datasets are freely available on Dryad and can be loaded as follows (Itter et al., 2018b).

```
# Download data archive
temp = tempfile()
download.file(paste("https://datadryad.org/bitstream/handle/10255/",
"dryad.195257/JEcol-2018-0266.R1.zip?sequence=1",sep=""),temp)

# Load tree growth data
tree.growth = read.csv(unz(temp,"JEcol-2018-0266.R1/West/TreeWest.csv"),
                       header = TRUE, stringsAsFactors = FALSE)
```

```
# Load ftc defoliation data
ftc.defol = read.csv(unz(temp,"JEcol-2018-0266.R1/West/DefolWest.csv"),
                     header = TRUE, stringsAsFactors = FALSE)

# Unlink data archive
unlink(temp)
```

Tree growth measurements are in the form of diameter increments ($\text{cm}\cdot\text{yr}^{-1}$) for individual trees. We convert these measurements to basal area increment ($\text{cm}^2 \cdot \text{yr}^{-1}$) and estimate mean annual basal area increment and tree age for all sampled aspen trees by study site.

```
# Define function to convert diameter (cm) to basal area (cm^2)
dbh2ba = function(d){
  (d^2)*(pi/4)
}

# Convert diameter to basal area in current and previous year
tree.growth$ba = dbh2ba(tree.growth$dbh)
tree.growth$ba.lag = dbh2ba(tree.growth$dbh.lag)

# Take difference between current and previous year basal area
# to estimate annual basal area increment (cm^2 per year)
tree.growth$bai = with(tree.growth, ba-ba.lag)

# Calculate mean annual basal area increment and age for
# sampled trembling aspen trees by study site (stand)
stand.vars = ddply(tree.growth[tree.growth$Species == "Potr",],
                   .(Stand,Year),summarize,
                   age = mean(age), gr = mean(bai))
```

The forest tent caterpillar defoliation data is ordinal with values 0 to 3 indicating none (0%), light (<35%), moderate (35-70%), and severe (>70%) defoliation levels, respectively. Previous studies have demonstrated boreal tree growth is affected by moderate-to-severe defoliation (see Itter et al., 2018a, for complete discussion). We convert the ordinal defoliation data to a binary variable (`ftc`) indicating the occurrence of moderate-to-severe defoliation events (`ftc = 1`, if `Defol` $>$ `1`; `ftc = 0`, if `Defol` $\leq$ `1`). The defoliation data is subset to select only those study sites where trembling aspen is present (the forest tent caterpillar host species). Finally, the model data frame (`boreal.dat`) is formed by joining the forest tent caterpillar disturbance chronology with the mean annual basal area increment estimates.

```
# Form binary moderate-to-severe defoliation variable
ftc.defol$ftc = with(ftc.defol, ifelse(Defol > 1, 1, 0))

# Identify study sites (stands) where trembling aspen
# is present
host.stands = sort(unique(
```

```
  tree.growth$Stand[tree.growth$Host == "Host"]))

# Subset defoliation data to include only host stands
ftc.defol = ftc.defol[ftc.defol$Stand %in% host.stands,]

# Form model data frame
boreal.dat = join(ftc.defol, stand.vars)
```

Mean annual basal area increment is modeled as a function of the occurrence of moderate-to-severe forest tent caterpillar defoliation events and mean tree age allowing for ecological memory to defoliation for up to 12 years before present.

```
# Fit ecological memory model
mod = ecomem(gr ~ age + ftc, data = boreal.dat, mem.vars = "ftc",
             L = 12, timeID = "Year", groupID = "Stand")
```

After assessing model convergence, we summarize the marginal posterior distributions for the ecological memory parameters. There is strong evidence of ecological memory in boreal tree growth responses to forest tent caterpillar defoliation. Posterior mean weight values greater than 0.01 exist for lags 0 to 8 reflecting persistent impacts of defoliation on mean annual basal area increment with defoliation in the current or previous year to growth having the greatest relative importance. Weighted defoliation event observations were negatively related to the mean annual basal area increment of aspen trees within study sites (Table B.1).

```
# Summarize marginal posterior distributions of model parameters
boreal.mem.summ = memsum(mod, verbose = FALSE)

# Print summary
kable(boreal.mem.summ, "latex", booktabs = TRUE, digits = 3,
caption="\\label{tab:memsum}Summary of marginal posterior
distributions for ecological memory model parameters generated
using the \\texttt{memsum()}
function.") %>%
  kable_styling(latex_options = c("striped", "hold_position"))
```

Finally, we plot the estimated ecological memory function for defoliation.

```
# Plot boreal tree growth memory to ftc defoliation
plotmem(mod)
```

Table B.1: Summary of marginal posterior distributions for ecological memory model parameters generated using the `memsum()` function.

| var | mean | median | q0.025 | q0.975 |
|---|---|---|---|---|
| (Intercept) | 4.563 | 4.561 | 4.400 | 4.740 |
| age | 0.010 | 0.010 | -0.149 | 0.168 |
| ftc | -4.838 | -4.817 | -5.922 | -3.813 |
| sig.y | 2.049 | 2.048 | 1.953 | 2.150 |
| ftc:w0 | 0.252 | 0.250 | 0.178 | 0.329 |
| ftc:w1 | 0.220 | 0.215 | 0.174 | 0.292 |
| ftc:w2 | 0.172 | 0.166 | 0.137 | 0.235 |
| ftc:w3 | 0.124 | 0.119 | 0.097 | 0.171 |
| ftc:w4 | 0.084 | 0.082 | 0.057 | 0.120 |
| ftc:w5 | 0.054 | 0.055 | 0.025 | 0.078 |
| ftc:w6 | 0.034 | 0.035 | 0.008 | 0.054 |
| ftc:w7 | 0.021 | 0.022 | 0.001 | 0.041 |
| ftc:w8 | 0.014 | 0.014 | 0.000 | 0.033 |
| ftc:w9 | 0.010 | 0.009 | 0.000 | 0.026 |
| ftc:w10 | 0.007 | 0.006 | 0.000 | 0.022 |
| ftc:w11 | 0.005 | 0.004 | 0.000 | 0.019 |
| ftc:w12 | 0.004 | 0.002 | 0.000 | 0.017 |

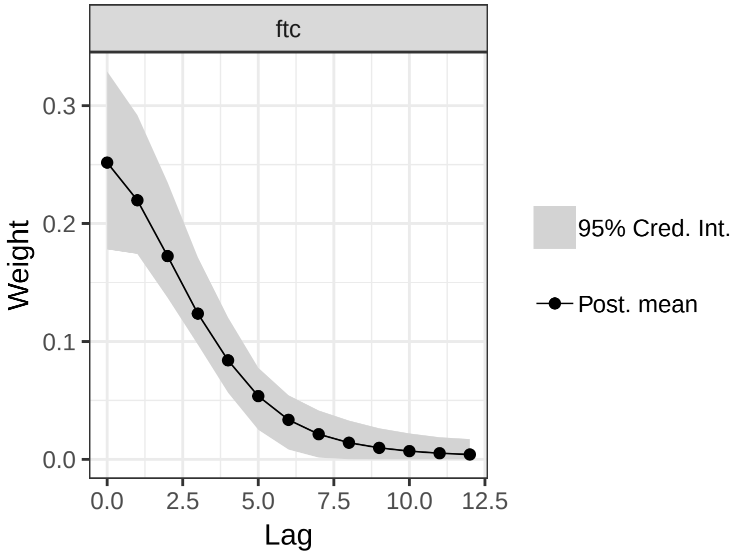


Figure B.5: Ecological memory of boreal tree growth to forest tent caterpillar defoliation events generated using the `plotmem()` function.

# References

Brandt, J., Flannigan, M., Maynard, D., Thompson, I., and Volney, W. (2013). An introduction to Canada's boreal zone: ecosystem processes, health, sustainability, and environmental issues 1. *Environmental Reviews*, 21(4):207–226.

Itter, M. S., D'Orangeville, L., Dawson, A., Kneeshaw, D., Duchesne, L., and Finley, A. O. (2018a). Boreal tree growth exhibits decadal-scale ecological memory to drought and insect defoliation, but no negative response to their interaction. *Journal of Ecology*. https://doi.org/0.1111/1365-2745.13087.

Itter, M. S., D'Orangeville, L., Dawson, A., Kneeshaw, D., Duchesne, L., and Finley, A. O. (2018b). Data from: Boreal tree growth exhibits decadal-scale ecological memory to drought and insect defoliation, but no negative response to their interaction. *Dryad Digital Repository*. https://doi.org/10.5061/dryad.f7bq534.

Knaus, J., Porzelius, C., Binder, H., and Schwarzer, G. (2009). Easier parallel computing in R with snowfall and sfCluster. *The R Journal*, 1(1):54–59.

Plummer, M., Best, N., Cowles, K., and Vines, K. (2006). CODA: Convergence diagnosis and output analysis for MCMC. *R News*, 6(1):7–11.

Tierney, L., Rossini, A. J., and Li, N. (2009). Snow: A parallel computing framework for the R system. *International Journal of Parallel Programming*, 37(1):78–90.

Wickham, H., Hester, J., and Chang, W. (2018). *devtools: Tools to Make Developing R Packages Easier*. R package version 2.0.1.
